# Supplementary material for: Multivariate Discrimination in Quantum Target Detection
Source: arXiv:2005.00612 ancillary file (2020-07-30)
Supplement: Supplementary file 1 [file supplementary.pdf]

# Supplementary Material: Multivariate Discrimination in Quantum Target Detection

Peter Svihra,[1,2,a)] Yingwen Zhang,[3] Paul Hockett,[3] Steven Ferrante,[4] Benjamin Sussman,[3,5] Duncan England,[3] and Andrei Nomerotski[4]

[1)] *Department of Physics, Faculty of Nuclear Sciences and Physical Engineering, Czech Technical University, Prague 115 19, Czech Republic*
[2)] *Department of Physics and Astronomy, School of Natural Sciences, University of Manchester, Manchester M13 9PL, United Kingdom*
[3)] *National Research Council of Canada, 100 Sussex Drive, Ottawa, Ontario, K1A 0R6, Canada*
[4)] *Physics Department, Brookhaven National Laboratory, Upton, NY 11973, USA*
[5)] *Department of Physics, University of Ottawa, Ottawa, Ontario, K1N 6N5, Canada*

(Dated: 30 July 2020)

## I. MONTE-CARLO MODEL

To study the signal and background separation using the likelihood ratio discriminant we developed a MC model tuned to the experimental conditions such as signal and background resolutions and rates. The simulated data contain spatial and temporal information about the single photon events in the camera accounting for all sources of photon pairing. Both signal and background events were generated independently and could be traced to determined origin of pairs in the coincidence algorithm. Below we provide more information on the model.

The SPDC process is simulated by generating events in pairs, the herald photon has a random $x_1$ coordinate along one stripe and the $x_2$ coordinate of the signal photon is calculated according to their energy correlation in the second stripe. After generating, the photon positions are smeared in $x$ and $y$ according to the optical resolution of the spectrometer. Further smearing in the $x$ coordinate is also introduced to account for the line width of the pump laser.

The spectral resolution can be determined from projections of the stripes onto $y$-axis, as shown in Figure S1 for real data and MC, both equivalent to 300 s of data taking. The left peak corresponds to the herald photon while the right peak corresponds to the signal photon, the latter peak is dominated by the jamming light background.

The ToA of the first photon was generated randomly, while the second photon has an identical ToA, smeared by a Gaussian resolution to account for the time resolution of the camera.

Experimental inefficiencies in the system such as target reflectively, fiber-coupling, and camera detection capabilities are included by introducing loss to the MC model and matching the MC rates of the signal and herald photons to the data.

The background MC simulates thermal noise of the intensifier as well as stray light in the system, the ToA and $x$, $y$ coordinates are randomly distributed. The jamming light is simulated only in the stripe with the signal photons representing background light from a jamming source collected by the telescope. The ToA is randomly distributed, and the position

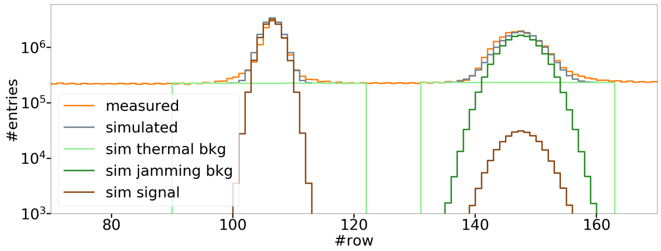


FIG. S1: Projections of the stripes on to the orthogonal axis. Comparison of measured and simulated data, see the text.

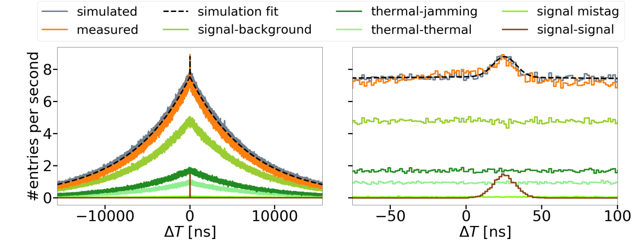


(a) Time difference $\Delta T$ distribution of photon pairs. Simulated data fit is obtained by Gaussian fit of signal-herald pairs and exponential fit of all backgrounds.

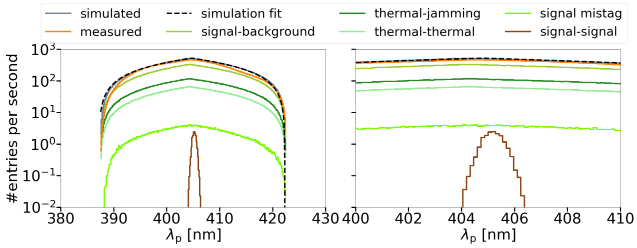


(b) Pump photon wavelength $\lambda_p$ distribution of the event pairs. Simulated data fit is obtained by Gaussian fit of signal-herald pairs and linear fit of all backgrounds.

FIG. S2: Signal and background rates of both measured and simulated data, after coincidence-finding algorithm. In the case of MC simulation, distributions are shown separately for all combinations of background (green diamonds of different shades) and of wanted signal (brown stars).

[a)] Electronic mail: peter.svihra@manchester.ac.uk

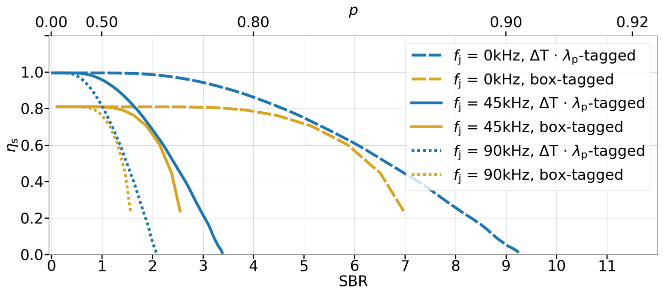


FIG. S3: Dependence of selection efficiency $\eta_s$ on SBR (bottom x-axis) and sample purity $p$ (top x-axis), compared performance of $\Delta T \cdot \lambda_p$-tagging and box-tagging for MC generated data of several jamming light rates. The measured rate in the experiment was 45 kHz.

is randomly distributed along the stripe and smeared in both directions in the same manner as the signal photons.

After generating the signal and background MC samples they were merged together in appropriate proportions to represent the corresponding rates. The nominal values for the herald and signal rates were 44.0 kHz and 0.88 kHz, respectively. This difference is predominantly due to losses when the signal photon scatters from the target. The uniformly distributed background rates were estimated at 200.0 kHz in the whole camera, and the jamming light contribution was determined to be 45.0 kHz, to give the best description of the experimental data. The quoted rates are for the registered photons with all detection inefficiencies already taken into account.

Figures S2a and S2b shows, correspondingly, distributions of the time difference $\Delta T$ for photon pairs and the pump photon wavelength $\lambda_p$. For the former case the MC distribution is fit by a Gaussian for the signal pairs and by an exponential function for the sum of all backgrounds. The time constant of the exponential for the background is consistent with the inverse of the total background rate as expected. The graphs compare the data and MC distributions, and also show separately different types of photon pairing in the MC case. Plots on the right side are zoomed-in versions of plots on the left side.

The photon pair energy is represented by the pump photon wavelength is plotted in Figure S2b for both data and MC. The energy was calculated using $x$ distributions of generated photons using random pairing for the background photons and exactly the same algorithm as for the real data. The MC distribution is fit by a Gaussian for the signal pairs and by a linear function for the sum of all backgrounds.

## II. DEPENDENCE ON BACKGROUND RATE AND RESOLUTION

An additional bonus of the MC model is that we can vary its parameters to predict how it affects the discriminant performance. This provides an easy and versatile way to explore parametric dependence of observables on experimental conditions, allowing to optimize the present and future experiments.

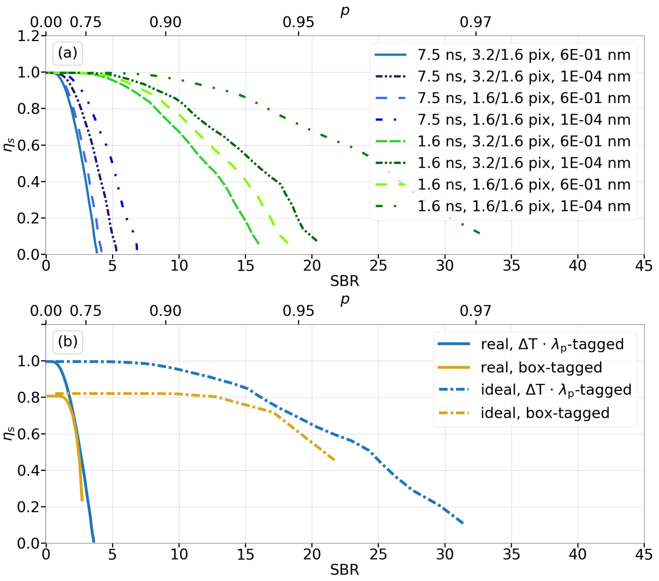


FIG. S4: Dependence of selection efficiency $\eta_s$ on SBR (bottom x-axis) and sample purity $p$ (top x-axis). **(a)** Compared performance of $\Delta T \cdot \lambda_p$-tagging for MC generated data: two values of time difference resolution $\sigma_{\Delta T}$ and four combinations of spectral resolution ( stripe-dependent $\sigma_{\lambda_{1,2}}$ and pump laser bandwidth $\Delta_\lambda$). The resolutions are specified in the same order in the legend with the top row corresponding to the real experimental setup. **(b)** Compared performance of $\Delta T \cdot \lambda_p$-tagging and box-tagging for the MC representation of real and ideal experimental setup (top and bottom row of legend in (a), respectively).

The dependence of efficiency on SBR and sample purity for several jamming light background rates is presented in Figure S3. The uniform background component due to the intensifier dark counts and stray light was not changed. The jamming light rate in the experimental data was 45 kHz. One can see a considerable effect of the background rate on the result. Increasing the jamming light rate to 90 kHz at the constant efficiency of 0.80 reduces the SBR by 39% while decreasing it to 0 kHz improves the ratio by 174%. The effects are consistent for both multivariate tagging methods, however, in all cases the combined discriminant outperforms the simple box-tagging method.

The dependence of efficiency on SBR and sample purity for several values of temporal and spectral resolution is presented in Figure S4(a). We assumed that all other experimental parameters did not change. It is clear that any improvement of the resolutions has significant impact on the performance. Improving the time resolution $\sigma_{\Delta T}$ to the limits of the camera, having the same smaller-sized fibers for both arms of the spectrometer and improving the line width $\Delta_\lambda$ of the pump laser results in the SBR improvement of the combined discriminant by 785% at the constant efficiency of 0.8, compared to the experiment. The 'ideal' best-case scenario for temporal and spectral resolution is compared to the 'real' resolu-

tions achieved in the experiment in Figure S4(b). We analyse each data set using $\Delta T \cdot \lambda_{\mathrm{p}}$-tagging and box-tagging methods showing that the optimal discriminant also outperforms with improved systematic resolution.
